# Supplementary material for: Linear Programming Based Near-Optimal Pricing for Laminar Bayesian Online Selection
Source: arXiv:1807.05477 source file (2024-03-08)
Supplement: Supplementary file 1 [file appendix.tex]

%\section{Deferred Proofs of \texorpdfstring{\Cref{sec:production-simple}}{TEXT}}

%\section{Deferred Proofs of \texorpdfstring{\Cref{sec:laminar}}{TEXT}}
%\section{Deferred Proofs of Section 2}
%\label{appendix:laminar-relaxation}
%\label{sec:exact-rounding}

%To complete the picture we now describe a simple online pricing scheme (with potentially randomized tie breaking) to round the solution of the linear program in \Cref{def:lp-optimal} in an online fashion. Our proposed rounding would be exact, which shows this linear program has no integrality gap and hence captures the optimal online policy. Moreover, the proposed rounding is clearly a polynomial time algorithm\footnote{Note however that the LP in \Cref{def:lp-optimal} has exponential size, both in the number of constraints and variables, and to the best of our knowledge there is no technique to solve it exactly.}, which we further use as a building block in our PTAS later in this section.

%\begin{definition}
%\label{def:pricing}
%An adaptive pricing with randomized tie breaking mechanism, defined by \emph{prices} $\T_t(\vec{r})$ and \emph{tie-break probabilities} $p_t(\vec{r})$, works as following:
%\begin{enumerate}
%\item At time $t$, it elicits the arriving customer value $v_t\sim F_t$.
%\item Given the vector of remaining capacities $\vec{r}$, compares $v_t$ with $\T_t(\vec{r})$.
%\item If $v_t>\T_t(\vec{r})$, serves the customer, and If $v_t<\T_t(\vec{r})$, it chooses to not serve the customer.
%\item In the case of a tie ($v_t=\T_t(\vec{r})$), it flips an independent coin with heads probability $p_t(\vec{r})$ and only serves the customer if the coin flips heads.  
% \end{enumerate}
%\end{definition}

%\begin{proposition}
%\label{prop:adaptive-pricing}
%There exists an adaptive pricing with a randomized tie breaking mechanism, as in \Cref{def:pricing}, whose expected social welfare is equal to the optimal solution of the linear program of optimal online policy in \Cref{def:lp-optimal}. 
%\end{proposition}








%
%\subsection{Discussion: extension to laminar over non-constant depth sub-problems.}
%As we saw earlier in \Cref{sec:laminar-mark}, we can prove the correctness of our polynomial time approximation scheme for general laminar matroids only if the depth of the laminar family is constant. At the same time, as an observation, if one thinks of the production constrained Bayesian selection problem as an instance of the laminar Bayesian selection, then the depth of the corresponding laminar family will simply be $T+1$, and hence is not a constant. Yet, as we saw, our approach in \cref{sec:production-simple} could also yield a PTAS. Can we still see this PTAS as a special case of our PTAS for the constant-depth laminar?
%
%This discrepancy can easily be explained by extending our result for the constant depth laminar Bayesian selection to a generalization where every element is replaced by a \emph{sub-problem}. With this view, in the production constrained Bayesian selection we indeed have only a 1-level tree (connecting the root to the type-specific sub-problems), and each leaf of this 1-level tree plays the role of one of the type-specific sub-problems. To make the analysis work, we require two things from each sub-problem. First, a local optimum online policy for each sub-problem, for possibly atomic or even non-positive value distributions, should be computable in polynomial time. Second, the selection rule of this local optimum online policy should satisfy the required negative cylinder dependency. Having these two properties, the proof of this section goes through, as by replacing each element with a group of negatively dependent elements we still have the required concentration. The proof of this generalization is basically the same, and so we omit to avoid redundancy.
